# Supplementary material for: Supporting Changes in Digital Ownership and Data Sovereignty Across the Automotive Value Chain with Catena-X
Source: arXiv:2406.07194 source file (2024-06-11)
Supplement: Supplementary file 1 [file fig99_appendix.tex]

% generated by Plantuml 1.2023.13      
\definecolor{plantucolor0000}{RGB}{0,0,0}
\definecolor{plantucolor0001}{RGB}{24,24,24}
\definecolor{plantucolor0002}{RGB}{226,226,240}
\definecolor{plantucolor0003}{RGB}{238,238,238}
\begin{tikzpicture}[yscale=-1
,pstyle0/.style={color=black,line width=1.5pt}
,pstyle1/.style={color=plantucolor0001,line width=0.5pt,dash pattern=on 5.0pt off 5.0pt}
,pstyle2/.style={color=plantucolor0001,fill=plantucolor0002,line width=0.5pt}
,pstyle3/.style={color=plantucolor0001,line width=1.0pt}
,pstyle4/.style={color=plantucolor0001,fill=plantucolor0001,line width=1.0pt}
]
\draw[pstyle0] (10pt,726.0123pt) rectangle (1214.6983pt,966.6604pt);
\draw[pstyle1] (67pt,39.0679pt) -- (67pt,1204.6026pt);
\draw[pstyle1] (216.3229pt,39.0679pt) -- (216.3229pt,1204.6026pt);
\draw[pstyle1] (364.8406pt,39.0679pt) -- (364.8406pt,1204.6026pt);
\draw[pstyle1] (684.0073pt,39.0679pt) -- (684.0073pt,1204.6026pt);
\draw[pstyle1] (824.634pt,39.0679pt) -- (824.634pt,1204.6026pt);
\draw[pstyle1] (1044.7593pt,39.0679pt) -- (1044.7593pt,1204.6026pt);
\draw[pstyle1] (1209.5421pt,39.0679pt) -- (1209.5421pt,1204.6026pt);
\draw[pstyle2] (20pt,10pt) arc (180:270:5pt) -- (25pt,5pt) -- (109.4676pt,5pt) arc (270:360:5pt) -- (114.4676pt,10pt) -- (114.4676pt,33.0679pt) arc (0:90:5pt) -- (109.4676pt,38.0679pt) -- (25pt,38.0679pt) arc (90:180:5pt) -- (20pt,33.0679pt) -- cycle;
\node at (27pt,12pt)[below right,color=black]{Supplier A};
\draw[pstyle2] (20pt,1208.6026pt) arc (180:270:5pt) -- (25pt,1203.6026pt) -- (109.4676pt,1203.6026pt) arc (270:360:5pt) -- (114.4676pt,1208.6026pt) -- (114.4676pt,1231.6705pt) arc (0:90:5pt) -- (109.4676pt,1236.6705pt) -- (25pt,1236.6705pt) arc (90:180:5pt) -- (20pt,1231.6705pt) -- cycle;
\node at (27pt,1210.6026pt)[below right,color=black]{Supplier A};
\draw[pstyle2] (169.3229pt,10pt) arc (180:270:5pt) -- (174.3229pt,5pt) -- (258.5515pt,5pt) arc (270:360:5pt) -- (263.5515pt,10pt) -- (263.5515pt,33.0679pt) arc (0:90:5pt) -- (258.5515pt,38.0679pt) -- (174.3229pt,38.0679pt) arc (90:180:5pt) -- (169.3229pt,33.0679pt) -- cycle;
\node at (176.3229pt,12pt)[below right,color=black]{Supplier B};
\draw[pstyle2] (169.3229pt,1208.6026pt) arc (180:270:5pt) -- (174.3229pt,1203.6026pt) -- (258.5515pt,1203.6026pt) arc (270:360:5pt) -- (263.5515pt,1208.6026pt) -- (263.5515pt,1231.6705pt) arc (0:90:5pt) -- (258.5515pt,1236.6705pt) -- (174.3229pt,1236.6705pt) arc (90:180:5pt) -- (169.3229pt,1231.6705pt) -- cycle;
\node at (176.3229pt,1210.6026pt)[below right,color=black]{Supplier B};
\draw[pstyle2] (318.8406pt,10pt) arc (180:270:5pt) -- (323.8406pt,5pt) -- (407.4406pt,5pt) arc (270:360:5pt) -- (412.4406pt,10pt) -- (412.4406pt,33.0679pt) arc (0:90:5pt) -- (407.4406pt,38.0679pt) -- (323.8406pt,38.0679pt) arc (90:180:5pt) -- (318.8406pt,33.0679pt) -- cycle;
\node at (325.8406pt,12pt)[below right,color=black]{Supplier C};
\draw[pstyle2] (318.8406pt,1208.6026pt) arc (180:270:5pt) -- (323.8406pt,1203.6026pt) -- (407.4406pt,1203.6026pt) arc (270:360:5pt) -- (412.4406pt,1208.6026pt) -- (412.4406pt,1231.6705pt) arc (0:90:5pt) -- (407.4406pt,1236.6705pt) -- (323.8406pt,1236.6705pt) arc (90:180:5pt) -- (318.8406pt,1231.6705pt) -- cycle;
\node at (325.8406pt,1210.6026pt)[below right,color=black]{Supplier C};
\draw[pstyle2] (659.0073pt,10pt) arc (180:270:5pt) -- (664.0073pt,5pt) -- (705.4073pt,5pt) arc (270:360:5pt) -- (710.4073pt,10pt) -- (710.4073pt,33.0679pt) arc (0:90:5pt) -- (705.4073pt,38.0679pt) -- (664.0073pt,38.0679pt) arc (90:180:5pt) -- (659.0073pt,33.0679pt) -- cycle;
\node at (666.0073pt,12pt)[below right,color=black]{OEM};
\draw[pstyle2] (659.0073pt,1208.6026pt) arc (180:270:5pt) -- (664.0073pt,1203.6026pt) -- (705.4073pt,1203.6026pt) arc (270:360:5pt) -- (710.4073pt,1208.6026pt) -- (710.4073pt,1231.6705pt) arc (0:90:5pt) -- (705.4073pt,1236.6705pt) -- (664.0073pt,1236.6705pt) arc (90:180:5pt) -- (659.0073pt,1231.6705pt) -- cycle;
\node at (666.0073pt,1210.6026pt)[below right,color=black]{OEM};
\draw[pstyle2] (778.634pt,10pt) arc (180:270:5pt) -- (783.634pt,5pt) -- (865.9988pt,5pt) arc (270:360:5pt) -- (870.9988pt,10pt) -- (870.9988pt,33.0679pt) arc (0:90:5pt) -- (865.9988pt,38.0679pt) -- (783.634pt,38.0679pt) arc (90:180:5pt) -- (778.634pt,33.0679pt) -- cycle;
\node at (785.634pt,12pt)[below right,color=black]{Consumer};
\draw[pstyle2] (778.634pt,1208.6026pt) arc (180:270:5pt) -- (783.634pt,1203.6026pt) -- (865.9988pt,1203.6026pt) arc (270:360:5pt) -- (870.9988pt,1208.6026pt) -- (870.9988pt,1231.6705pt) arc (0:90:5pt) -- (865.9988pt,1236.6705pt) -- (783.634pt,1236.6705pt) arc (90:180:5pt) -- (778.634pt,1231.6705pt) -- cycle;
\node at (785.634pt,1210.6026pt)[below right,color=black]{Consumer};
\draw[pstyle2] (990.7593pt,10pt) arc (180:270:5pt) -- (995.7593pt,5pt) -- (1094.0617pt,5pt) arc (270:360:5pt) -- (1099.0617pt,10pt) -- (1099.0617pt,33.0679pt) arc (0:90:5pt) -- (1094.0617pt,38.0679pt) -- (995.7593pt,38.0679pt) arc (90:180:5pt) -- (990.7593pt,33.0679pt) -- cycle;
\node at (997.7593pt,12pt)[below right,color=black]{Repair Shop};
\draw[pstyle2] (990.7593pt,1208.6026pt) arc (180:270:5pt) -- (995.7593pt,1203.6026pt) -- (1094.0617pt,1203.6026pt) arc (270:360:5pt) -- (1099.0617pt,1208.6026pt) -- (1099.0617pt,1231.6705pt) arc (0:90:5pt) -- (1094.0617pt,1236.6705pt) -- (995.7593pt,1236.6705pt) arc (90:180:5pt) -- (990.7593pt,1231.6705pt) -- cycle;
\node at (997.7593pt,1210.6026pt)[below right,color=black]{Repair Shop};
\draw[pstyle2] (1160.5421pt,10pt) arc (180:270:5pt) -- (1165.5421pt,5pt) -- (1253.8545pt,5pt) arc (270:360:5pt) -- (1258.8545pt,10pt) -- (1258.8545pt,33.0679pt) arc (0:90:5pt) -- (1253.8545pt,38.0679pt) -- (1165.5421pt,38.0679pt) arc (90:180:5pt) -- (1160.5421pt,33.0679pt) -- cycle;
\node at (1167.5421pt,12pt)[below right,color=black]{Dismantler};
\draw[pstyle2] (1160.5421pt,1208.6026pt) arc (180:270:5pt) -- (1165.5421pt,1203.6026pt) -- (1253.8545pt,1203.6026pt) arc (270:360:5pt) -- (1258.8545pt,1208.6026pt) -- (1258.8545pt,1231.6705pt) arc (0:90:5pt) -- (1253.8545pt,1236.6705pt) -- (1165.5421pt,1236.6705pt) arc (90:180:5pt) -- (1160.5421pt,1231.6705pt) -- cycle;
\node at (1167.5421pt,1210.6026pt)[below right,color=black]{Dismantler};
\draw[pstyle3] (67.2338pt,90.4799pt) -- (109.2338pt,90.4799pt);
\draw[pstyle3] (109.2338pt,90.4799pt) -- (109.2338pt,103.4799pt);
\draw[pstyle3] (68.2338pt,103.4799pt) -- (109.2338pt,103.4799pt);
\draw[pstyle4] (78.2338pt,99.4799pt) -- (68.2338pt,103.4799pt) -- (78.2338pt,107.4799pt) -- (74.2338pt,103.4799pt) -- cycle;
\node at (74.2338pt,53.0679pt)[below right,color=black]{Create Digital Twin};
\node at (74.2338pt,70.7739pt)[below right,color=black]{ of component A};
\draw[pstyle4] (672.7073pt,148.892pt) -- (682.7073pt,152.892pt) -- (672.7073pt,156.892pt) -- (676.7073pt,152.892pt) -- cycle;
\draw[pstyle3] (67.2338pt,152.892pt) -- (678.7073pt,152.892pt);
\node at (74.2338pt,115.4799pt)[below right,color=black]{Send component and link to Digital Twins};
\node at (74.2338pt,133.186pt)[below right,color=black]{ of component A for BOM of vehicle};
\draw[pstyle3] (216.4372pt,202.304pt) -- (258.4372pt,202.304pt);
\draw[pstyle3] (258.4372pt,202.304pt) -- (258.4372pt,215.304pt);
\draw[pstyle3] (217.4372pt,215.304pt) -- (258.4372pt,215.304pt);
\draw[pstyle4] (227.4372pt,211.304pt) -- (217.4372pt,215.304pt) -- (227.4372pt,219.304pt) -- (223.4372pt,215.304pt) -- cycle;
\node at (223.4372pt,164.892pt)[below right,color=black]{Create Digital Twin};
\node at (223.4372pt,182.598pt)[below right,color=black]{ of component B};
\draw[pstyle4] (672.7073pt,260.716pt) -- (682.7073pt,264.716pt) -- (672.7073pt,268.716pt) -- (676.7073pt,264.716pt) -- cycle;
\draw[pstyle3] (216.4372pt,264.716pt) -- (678.7073pt,264.716pt);
\node at (223.4372pt,227.304pt)[below right,color=black]{Send component and link to Digital Twins};
\node at (223.4372pt,245.01pt)[below right,color=black]{ of component B for BOM of vehicle};
\draw[pstyle3] (365.6406pt,314.1281pt) -- (407.6406pt,314.1281pt);
\draw[pstyle3] (407.6406pt,314.1281pt) -- (407.6406pt,327.1281pt);
\draw[pstyle3] (366.6406pt,327.1281pt) -- (407.6406pt,327.1281pt);
\draw[pstyle4] (376.6406pt,323.1281pt) -- (366.6406pt,327.1281pt) -- (376.6406pt,331.1281pt) -- (372.6406pt,327.1281pt) -- cycle;
\node at (372.6406pt,276.716pt)[below right,color=black]{Create Digital Twin};
\node at (372.6406pt,294.4221pt)[below right,color=black]{ of component C};
\draw[pstyle4] (672.7073pt,372.5401pt) -- (682.7073pt,376.5401pt) -- (672.7073pt,380.5401pt) -- (676.7073pt,376.5401pt) -- cycle;
\draw[pstyle3] (365.6406pt,376.5401pt) -- (678.7073pt,376.5401pt);
\node at (372.6406pt,339.1281pt)[below right,color=black]{Send component and link to Digital Twins};
\node at (372.6406pt,356.8341pt)[below right,color=black]{ of component C for BOM of vehicle};
\draw[pstyle3] (684.7073pt,425.9521pt) -- (726.7073pt,425.9521pt);
\draw[pstyle3] (726.7073pt,425.9521pt) -- (726.7073pt,438.9521pt);
\draw[pstyle3] (685.7073pt,438.9521pt) -- (726.7073pt,438.9521pt);
\draw[pstyle4] (695.7073pt,434.9521pt) -- (685.7073pt,438.9521pt) -- (695.7073pt,442.9521pt) -- (691.7073pt,438.9521pt) -- cycle;
\node at (691.7073pt,388.5401pt)[below right,color=black]{Manufacture};
\node at (691.7073pt,406.2461pt)[below right,color=black]{ vehicle};
\draw[pstyle3] (684.7073pt,506.0702pt) -- (726.7073pt,506.0702pt);
\draw[pstyle3] (726.7073pt,506.0702pt) -- (726.7073pt,519.0702pt);
\draw[pstyle3] (685.7073pt,519.0702pt) -- (726.7073pt,519.0702pt);
\draw[pstyle4] (695.7073pt,515.0702pt) -- (685.7073pt,519.0702pt) -- (695.7073pt,523.0702pt) -- (691.7073pt,519.0702pt) -- cycle;
\node at (691.7073pt,450.9521pt)[below right,color=black]{Generate};
\node at (691.7073pt,468.6582pt)[below right,color=black]{ Digital Twin};
\node at (691.7073pt,486.3642pt)[below right,color=black]{ of vehicle};
\draw[pstyle3] (684.7073pt,603.8943pt) -- (726.7073pt,603.8943pt);
\draw[pstyle3] (726.7073pt,603.8943pt) -- (726.7073pt,616.8943pt);
\draw[pstyle3] (685.7073pt,616.8943pt) -- (726.7073pt,616.8943pt);
\draw[pstyle4] (695.7073pt,612.8943pt) -- (685.7073pt,616.8943pt) -- (695.7073pt,620.8943pt) -- (691.7073pt,616.8943pt) -- cycle;
\node at (691.7073pt,531.0702pt)[below right,color=black]{Integrate};
\node at (691.7073pt,548.7762pt)[below right,color=black]{ Digital Twins};
\node at (691.7073pt,566.4822pt)[below right,color=black]{ of components in};
\node at (691.7073pt,584.1882pt)[below right,color=black]{ BoM of vehicle};
\draw[pstyle4] (812.8164pt,662.3063pt) -- (822.8164pt,666.3063pt) -- (812.8164pt,670.3063pt) -- (816.8164pt,666.3063pt) -- cycle;
\draw[pstyle3] (684.7073pt,666.3063pt) -- (818.8164pt,666.3063pt);
\node at (691.7073pt,628.8943pt)[below right,color=black]{sell};
\node at (691.7073pt,646.6003pt)[below right,color=black]{ vehicle};
\draw[pstyle3] (824.8164pt,698.0123pt) -- (866.8164pt,698.0123pt);
\draw[pstyle3] (866.8164pt,698.0123pt) -- (866.8164pt,711.0123pt);
\draw[pstyle3] (825.8164pt,711.0123pt) -- (866.8164pt,711.0123pt);
\draw[pstyle4] (835.8164pt,707.0123pt) -- (825.8164pt,711.0123pt) -- (835.8164pt,715.0123pt) -- (831.8164pt,711.0123pt) -- cycle;
\node at (831.8164pt,678.3063pt)[below right,color=black]{use vehicle};
\draw[color=black,fill=plantucolor0003,line width=1.5pt] (10pt,726.0123pt) -- (89.199pt,726.0123pt) -- (89.199pt,735.7183pt) -- (79.199pt,745.7183pt) -- (10pt,745.7183pt) -- (10pt,726.0123pt);
\draw[pstyle0] (10pt,726.0123pt) rectangle (1214.6983pt,966.6604pt);
\node at (25pt,727.0123pt)[below right,color=black]{\textbf{loop}};
\node at (104.199pt,728.0123pt)[below right,color=black]{\textbf{[for usage whenever the vehicle is malfunctioning or component A, B or C have to be maintained]}};
\draw[pstyle4] (1032.9105pt,765.4243pt) -- (1042.9105pt,769.4243pt) -- (1032.9105pt,773.4243pt) -- (1036.9105pt,769.4243pt) -- cycle;
\draw[pstyle3] (824.8164pt,769.4243pt) -- (1038.9105pt,769.4243pt);
\node at (831.8164pt,749.7183pt)[below right,color=black]{bring vehicle to repair shop};
\draw[pstyle3] (1044.9105pt,818.8364pt) -- (1086.9105pt,818.8364pt);
\draw[pstyle3] (1086.9105pt,818.8364pt) -- (1086.9105pt,831.8364pt);
\draw[pstyle3] (1045.9105pt,831.8364pt) -- (1086.9105pt,831.8364pt);
\draw[pstyle4] (1055.9105pt,827.8364pt) -- (1045.9105pt,831.8364pt) -- (1055.9105pt,835.8364pt) -- (1051.9105pt,831.8364pt) -- cycle;
\node at (1051.9105pt,781.4243pt)[below right,color=black]{exchange component};
\node at (1051.9105pt,799.1304pt)[below right,color=black]{ or overhaul them};
\draw[pstyle4] (695.7073pt,859.5424pt) -- (685.7073pt,863.5424pt) -- (695.7073pt,867.5424pt) -- (691.7073pt,863.5424pt) -- cycle;
\draw[pstyle3] (689.7073pt,863.5424pt) -- (1043.9105pt,863.5424pt);
\node at (701.7073pt,843.8364pt)[below right,color=black]{update vehicle Digital Twin};
\draw[pstyle4] (78.2338pt,891.2484pt) -- (68.2338pt,895.2484pt) -- (78.2338pt,899.2484pt) -- (74.2338pt,895.2484pt) -- cycle;
\draw[pstyle3] (72.2338pt,895.2484pt) -- (1043.9105pt,895.2484pt);
\node at (84.2338pt,875.5424pt)[below right,color=black]{update component A};
\draw[pstyle4] (227.4372pt,922.9544pt) -- (217.4372pt,926.9544pt) -- (227.4372pt,930.9544pt) -- (223.4372pt,926.9544pt) -- cycle;
\draw[pstyle3] (221.4372pt,926.9544pt) -- (1043.9105pt,926.9544pt);
\node at (233.4372pt,907.2484pt)[below right,color=black]{update component B};
\draw[pstyle4] (376.6406pt,954.6604pt) -- (366.6406pt,958.6604pt) -- (376.6406pt,962.6604pt) -- (372.6406pt,958.6604pt) -- cycle;
\draw[pstyle3] (370.6406pt,958.6604pt) -- (1043.9105pt,958.6604pt);
\node at (382.6406pt,938.9544pt)[below right,color=black]{update component C};
\draw[pstyle4] (1197.6983pt,993.3665pt) -- (1207.6983pt,997.3665pt) -- (1197.6983pt,1001.3665pt) -- (1201.6983pt,997.3665pt) -- cycle;
\draw[pstyle3] (824.8164pt,997.3665pt) -- (1203.6983pt,997.3665pt);
\node at (831.8164pt,977.6604pt)[below right,color=black]{bring vehicle to dismatler};
\draw[pstyle3] (1209.6983pt,1046.7785pt) -- (1251.6983pt,1046.7785pt);
\draw[pstyle3] (1251.6983pt,1046.7785pt) -- (1251.6983pt,1059.7785pt);
\draw[pstyle3] (1210.6983pt,1059.7785pt) -- (1251.6983pt,1059.7785pt);
\draw[pstyle4] (1220.6983pt,1055.7785pt) -- (1210.6983pt,1059.7785pt) -- (1220.6983pt,1063.7785pt) -- (1216.6983pt,1059.7785pt) -- cycle;
\node at (1216.6983pt,1009.3665pt)[below right,color=black]{initiate };
\node at (1216.6983pt,1027.0725pt)[below right,color=black]{EoL certificates};
\draw[pstyle4] (78.2338pt,1087.4845pt) -- (68.2338pt,1091.4845pt) -- (78.2338pt,1095.4845pt) -- (74.2338pt,1091.4845pt) -- cycle;
\draw[pstyle3] (72.2338pt,1091.4845pt) -- (1208.6983pt,1091.4845pt);
\node at (84.2338pt,1071.7785pt)[below right,color=black]{update component A as EoL};
\draw[pstyle4] (227.4372pt,1119.1905pt) -- (217.4372pt,1123.1905pt) -- (227.4372pt,1127.1905pt) -- (223.4372pt,1123.1905pt) -- cycle;
\draw[pstyle3] (221.4372pt,1123.1905pt) -- (1208.6983pt,1123.1905pt);
\node at (233.4372pt,1103.4845pt)[below right,color=black]{update component B as EoL};
\draw[pstyle4] (376.6406pt,1150.8965pt) -- (366.6406pt,1154.8965pt) -- (376.6406pt,1158.8965pt) -- (372.6406pt,1154.8965pt) -- cycle;
\draw[pstyle3] (370.6406pt,1154.8965pt) -- (1208.6983pt,1154.8965pt);
\node at (382.6406pt,1135.1905pt)[below right,color=black]{update component C as EoL};
\draw[pstyle4] (695.7073pt,1182.6026pt) -- (685.7073pt,1186.6026pt) -- (695.7073pt,1190.6026pt) -- (691.7073pt,1186.6026pt) -- cycle;
\draw[pstyle3] (689.7073pt,1186.6026pt) -- (1208.6983pt,1186.6026pt);
\node at (701.7073pt,1166.8965pt)[below right,color=black]{update vehicle as EoL};
\end{tikzpicture}
